# Supplementary material for: Exotica in the Globular Cluster M4, Studied with Chandra, HST, and the VLA
Source: arXiv:2306.11770 ancillary file (2023-06-20)
Supplement: Supplementary file 1 [file M4_Appendix_B.pdf]

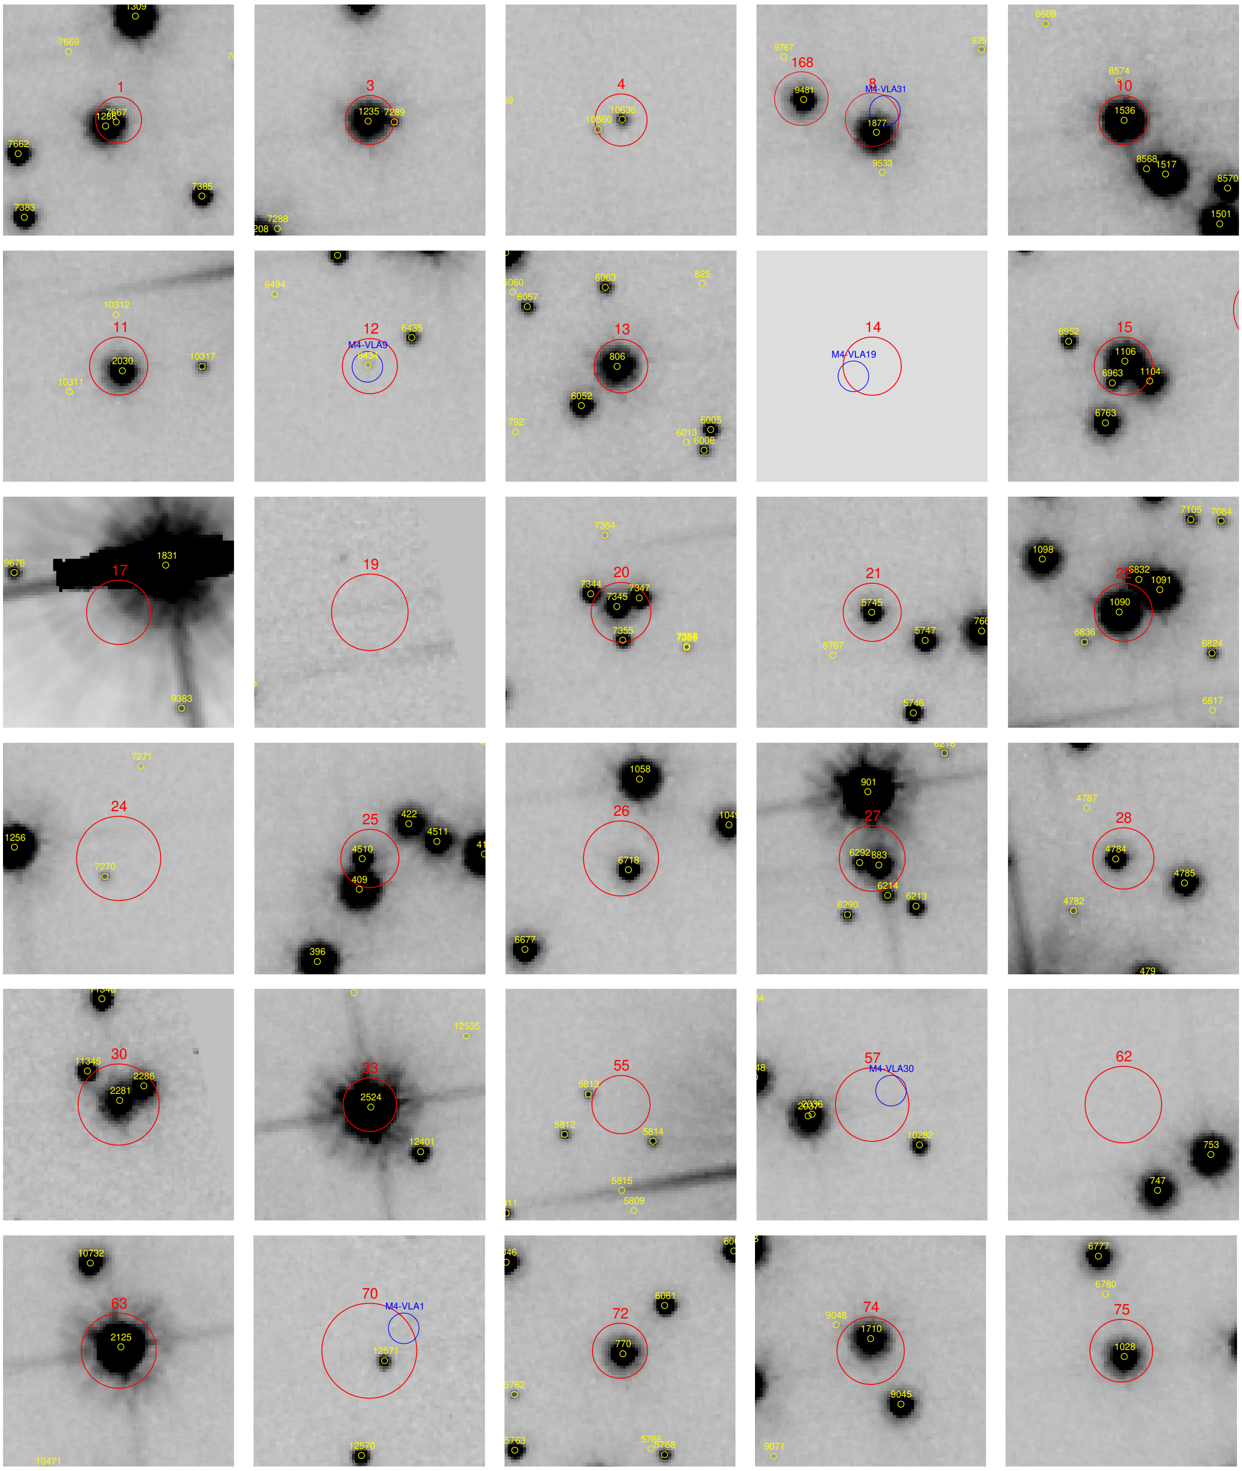

**Figure B1:** Finding charts: CX1 – CX75. All charts are for the $V_{606}$ band images from the HUGS project. The field size is 3 arcsec on a side, with N up and E to the left. Only objects that lie within the HUGS FoV or for which there is a coincidence with a MAVERIC radio source (indicated by a blue circle of radius 0.2 arcsec) are shown. In most cases, there is at most one object within the error circle (indicated in red). In nearly every case, the object closest to the centre of the error circle is the counterpart. In the following cases where there are multiple objects within the error circle, the counterparts are: CX1 – 7667, CX3 – 1235, CX4 – 10636, CX15 – 1106, CX20 – 7345, CX27 – 883, and CX30 – 2281.

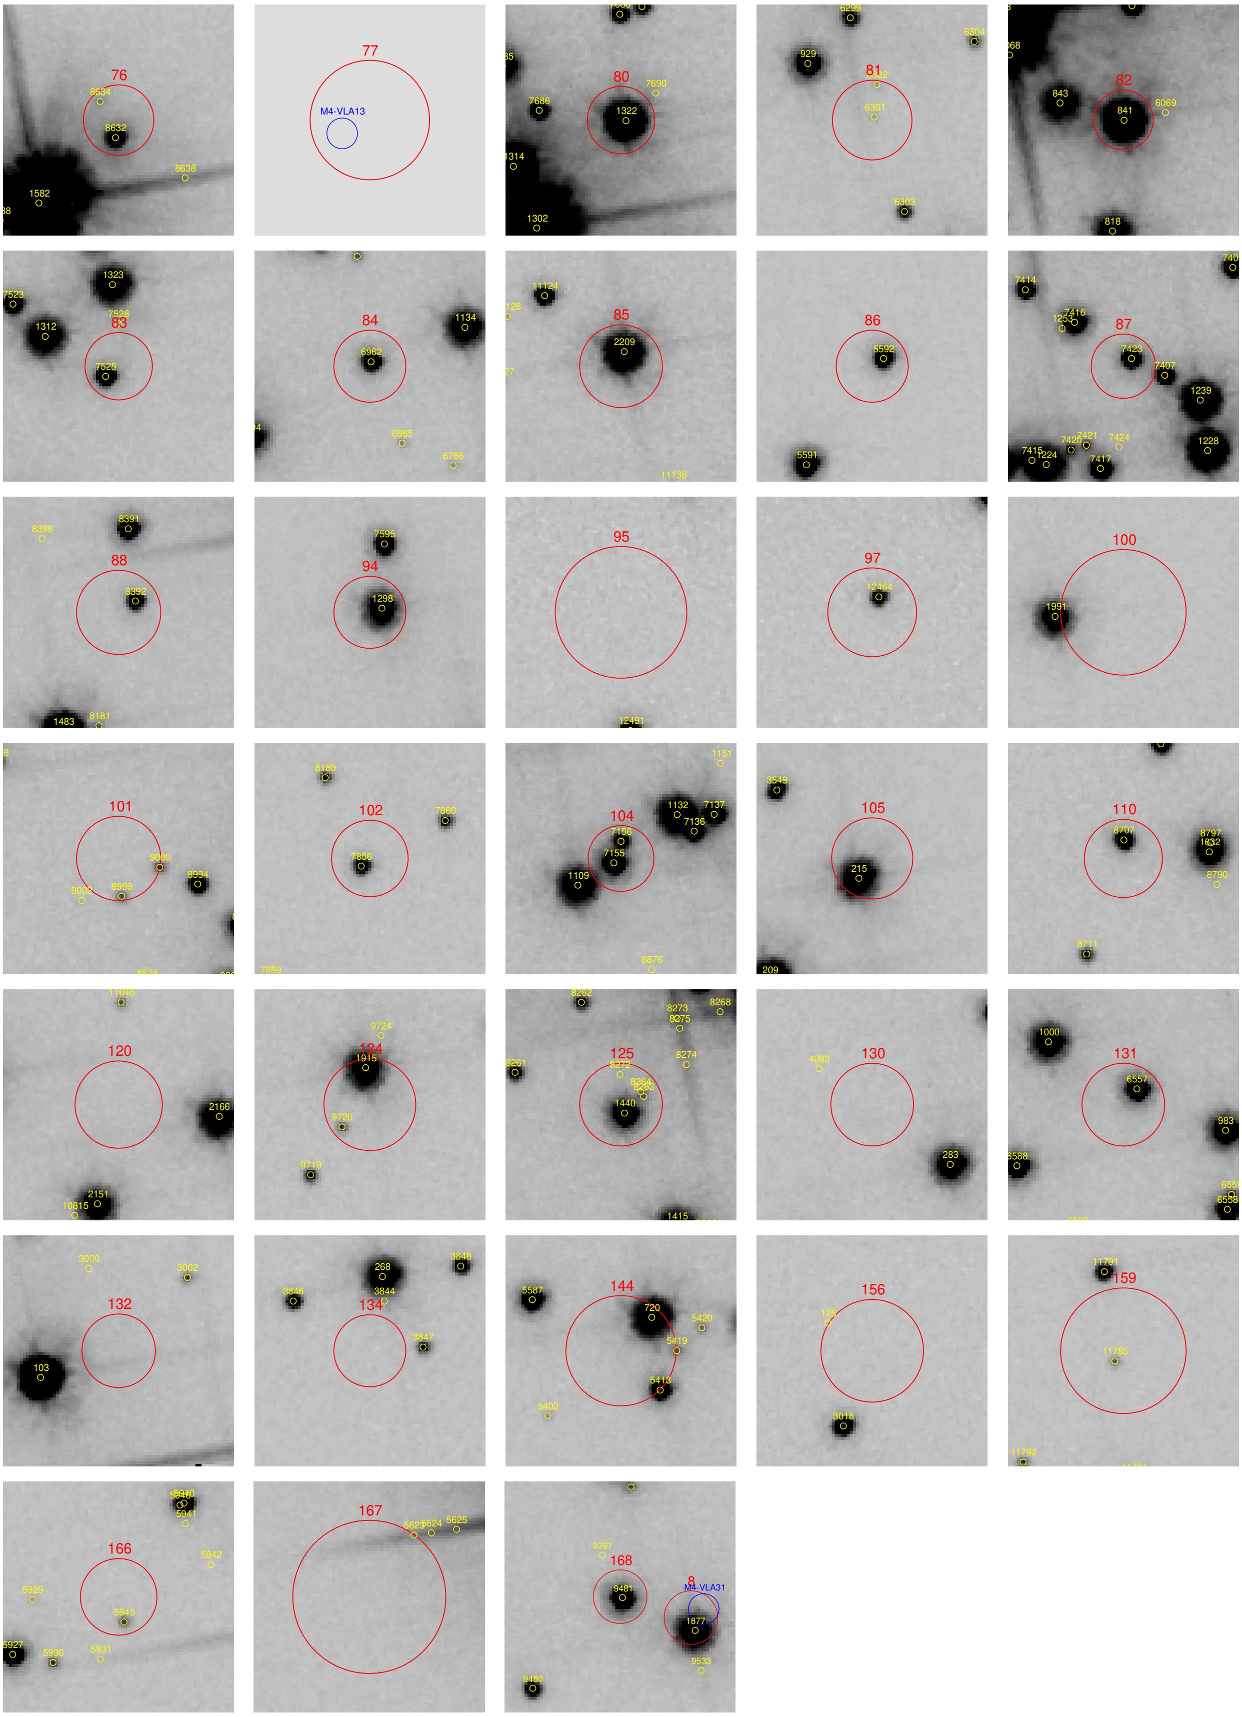


**Figure B2:** Finding charts: CX76 – CX168, as in Fig. B1. In the following cases where there are multiple objects within the error circle, the counterparts are: CX76 – 8632, CX81 – 6301, CX101 – 8999, CX104 – 7155, CX124 – 1915, CX125 – 1440, and CX144 – 720.
